# Supplementary material for: How volatilities nonlocal in time affect the price dynamics in complex financial systems
Source: arXiv:1502.00824 source file (2015-02-03)
Supplement: Supplementary file 1 [file S1_Appendix.pdf]

## S1 Appendix

### Calculation for $P^+(t)|_{\Delta v(t') > 0}$ , $P^+(t)|_{\Delta v(t') < 0}$ and $P_0(t)$ , and relation among them

We present the calculation for  $P^+(t)|_{\Delta v(t') > 0}$ ,  $P^+(t)|_{\Delta v(t') < 0}$  and  $P_0(t)$ , and derive the relation among them.

#### Calculation for $P^+(t)|_{\Delta v(t') > 0}$ , $P^+(t)|_{\Delta v(t') < 0}$ and $P_0(t)$

The length of the time series is denoted by  $T$ . According to the definition of  $\Delta v(t')$ ,  $T_2$  is the long time window. In the calculation,  $t'$  should satisfy  $t' - T_2 \geq 0$  and  $t' + t \leq T$ . With  $t'$  ranging from  $T_2$  to  $T - t$ , we count the number of the following cases:

- (a)  $\Delta v(t') > 0$  and  $r(t' + t) > 0$  ;
- (b)  $\Delta v(t') > 0$  and  $r(t' + t) < 0$  ;
- (c)  $\Delta v(t') < 0$  and  $r(t' + t) > 0$  ;
- (d)  $\Delta v(t') < 0$  and  $r(t' + t) < 0$  ,

and denote them by  $n_{\Delta v+}^{r+}$ ,  $n_{\Delta v+}^{r-}$ ,  $n_{\Delta v-}^{r+}$  and  $n_{\Delta v-}^{r-}$ , respectively.

From the definition of the normalized logarithmic return,  $r(t' + t)$  and  $\Delta v(t')$  are almost impossible to be zero. Having examined the data, we confirm that there are no data points with  $\Delta v(t') = 0$  or  $r(t' + t) = 0$  in the time series we analyze.

Then the probability of  $r(t' + t) > 0$  on the condition of  $\Delta v(t') > 0$  is

$$P^+(t)|_{\Delta v(t') > 0} = \frac{n_{\Delta v+}^{r+}}{n_{\Delta v+}^{r+} + n_{\Delta v+}^{r-}} ,$$

and the probability of  $r(t' + t) > 0$  on the condition of  $\Delta v(t') < 0$  is

$$P^+(t)|_{\Delta v(t') < 0} = \frac{n_{\Delta v-}^{r+}}{n_{\Delta v-}^{r+} + n_{\Delta v-}^{r-}} .$$

The unconditional probability  $P_0(t)$  is

$$P_0(t) = \frac{n_{\Delta v+}^{r+} + n_{\Delta v-}^{r+}}{n_{\Delta v+}^{r+} + n_{\Delta v-}^{r+} + n_{\Delta v+}^{r-} + n_{\Delta v-}^{r-}} .$$

**Relation among  $P^+(t)|_{\Delta v(t)>0}$ ,  $P^+(t)|_{\Delta v(t)<0}$  and  $P_0(t)$**

$$P^+(t)|_{\Delta v(t)>0} - P_0(t) = \frac{n_{\Delta v+}^{r+} n_{\Delta v-}^{r-} - n_{\Delta v-}^{r+} n_{\Delta v+}^{r-}}{(n_{\Delta v+}^{r+} + n_{\Delta v+}^{r-})(n_{\Delta v+}^{r+} + n_{\Delta v-}^{r+} + n_{\Delta v+}^{r-} + n_{\Delta v-}^{r-})}.$$

$$P^+(t)|_{\Delta v(t)<0} - P_0(t) = \frac{n_{\Delta v-}^{r+} n_{\Delta v+}^{r-} - n_{\Delta v+}^{r+} n_{\Delta v-}^{r-}}{(n_{\Delta v-}^{r+} + n_{\Delta v-}^{r-})(n_{\Delta v+}^{r+} + n_{\Delta v-}^{r+} + n_{\Delta v+}^{r-} + n_{\Delta v-}^{r-})}.$$

If  $P^+(t)|_{\Delta v(t)>0} - P_0(t) = 0$  or  $P^+(t)|_{\Delta v(t)<0} - P_0(t) = 0$ ,

we have  $n_{\Delta v+}^{r+} n_{\Delta v-}^{r-} - n_{\Delta v-}^{r+} n_{\Delta v+}^{r-} = 0$ .

Therefore,  $P^+(t)|_{\Delta v(t)>0} = P^+(t)|_{\Delta v(t)<0} = P_0(t)$ .

If  $P^+(t)|_{\Delta v(t)>0} - P_0(t) \neq 0$ , we have

$$\begin{aligned} & [P^+(t)|_{\Delta v(t)>0} - P_0(t)] \cdot [P^+(t)|_{\Delta v(t)<0} - P_0(t)] \\ &= \frac{-(n_{\Delta v-}^{r+} n_{\Delta v+}^{r-} - n_{\Delta v+}^{r+} n_{\Delta v-}^{r-})^2}{(n_{\Delta v+}^{r+} + n_{\Delta v+}^{r-})(n_{\Delta v-}^{r+} + n_{\Delta v-}^{r-})(n_{\Delta v+}^{r+} + n_{\Delta v-}^{r+} + n_{\Delta v+}^{r-} + n_{\Delta v-}^{r-})^2} < 0. \end{aligned}$$

Therefore,

if  $P^+(t)|_{\Delta v(t)>0} - P_0(t) > 0$ , we have  $P^+(t)|_{\Delta v(t)<0} - P_0(t) < 0$ ;

if  $P^+(t)|_{\Delta v(t)>0} - P_0(t) < 0$ , we have  $P^+(t)|_{\Delta v(t)<0} - P_0(t) > 0$ .
